# Supplementary material for: 3D Compression Using Neural Fields
Source: arXiv:2311.13009 source file (2023-11-21)
Supplement: Supplementary file 1 [file 6_supplement.tex]

\\
\\
We provide supporting materials for our main work. \autoref{sec:ablation} reports additional ablation studies of our method and the baselines. In \autoref{sec:experimental_details}, we provide additional details for the experiments conducted in the main paper. Lastly, \autoref{sec:qualitative_results} shows additional qualitative examples of reconstructed shapes of \acp{nf} and the baselines. 

\section{Ablation Studies}\label{sec:ablation}

We provide additional insights into \ac{nf}-based 3D compression. \autoref{ssec:ablation_bitwidth} analyses the impact of the bitwidth $b$ used for quantizing \acp{nf}. In \autoref{ssec:ablation_l1}, we ablate the impact of $\ell 1$-regularization on the \stanford{}. \autoref{ssec:ablation_activation} compares the use of the abs activation function in \acp{udf} with the ReLU activation function and \autoref{ssec:ablation_num_points} investigates the behaviour of each method for varying size of the \ac{pc}. In \autoref{ssec:ablation_geom_attr}, we demonstrate that sequentially compressing geometry and attributes outperforms joint training and \autoref{ssec:ablation_mc_grid} analyses the impact of the grid resolution used for extracting meshes from \acp{nf} using \ac{mc}. Lastly, \autoref{ssec:udf_fluctuation} demonstrates that the parameter initialization has the largest impact on the fluctuation of the performance of \acp{udf}.

\begin{figure}[b!]
\centering
\setlength{\tabcolsep}{1pt}
\begin{tabular}{ccc}
\includegraphics[width=\fourPlotsSizeWithLabel]{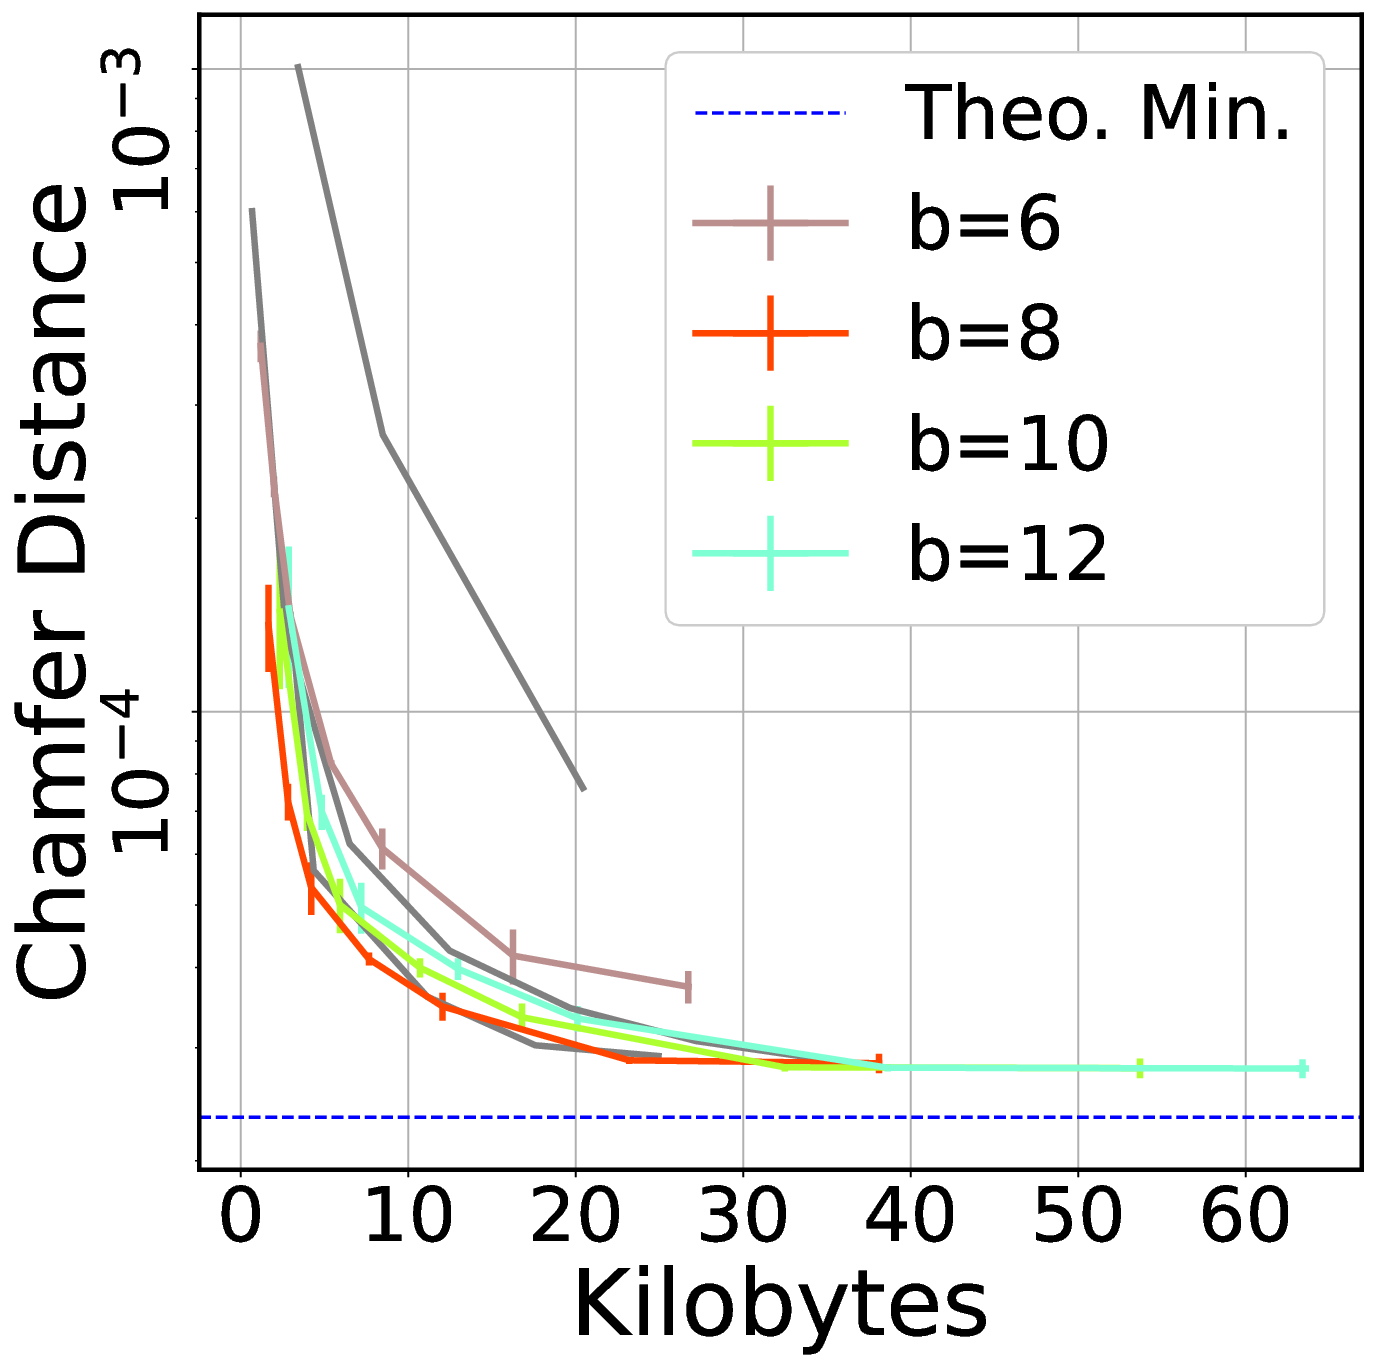} & 
\includegraphics[width=\fourPlotsSize]{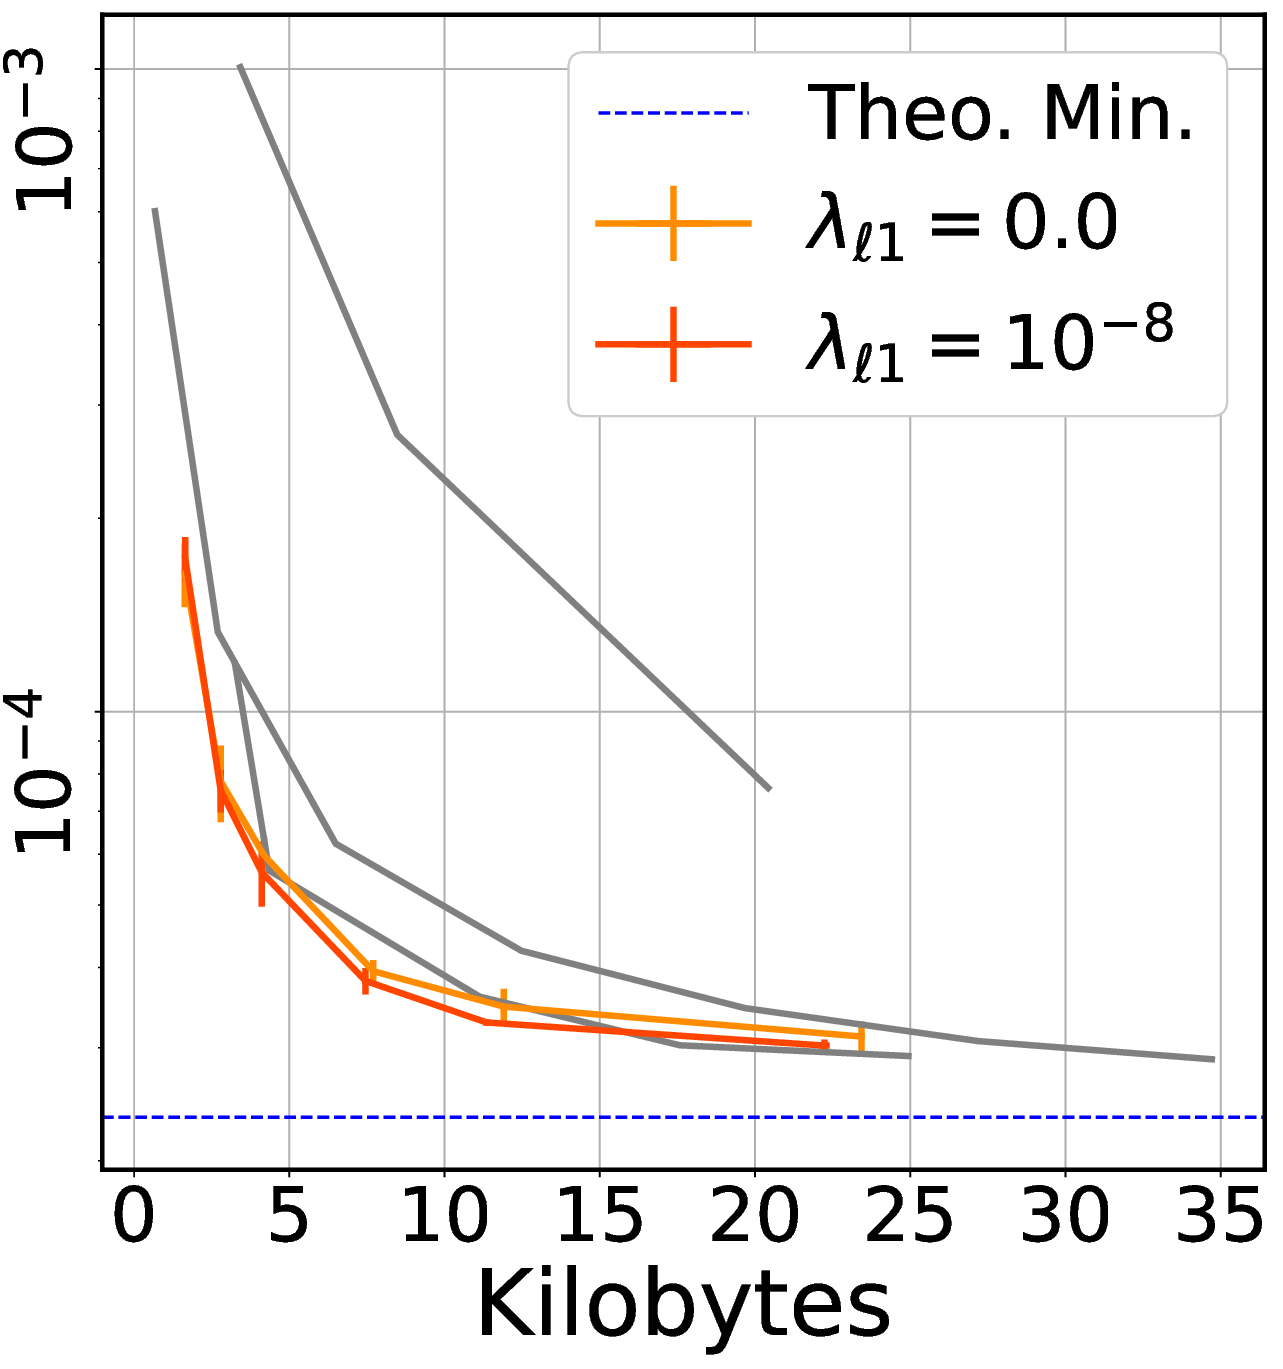} &
\includegraphics[width=\fourPlotsSize]{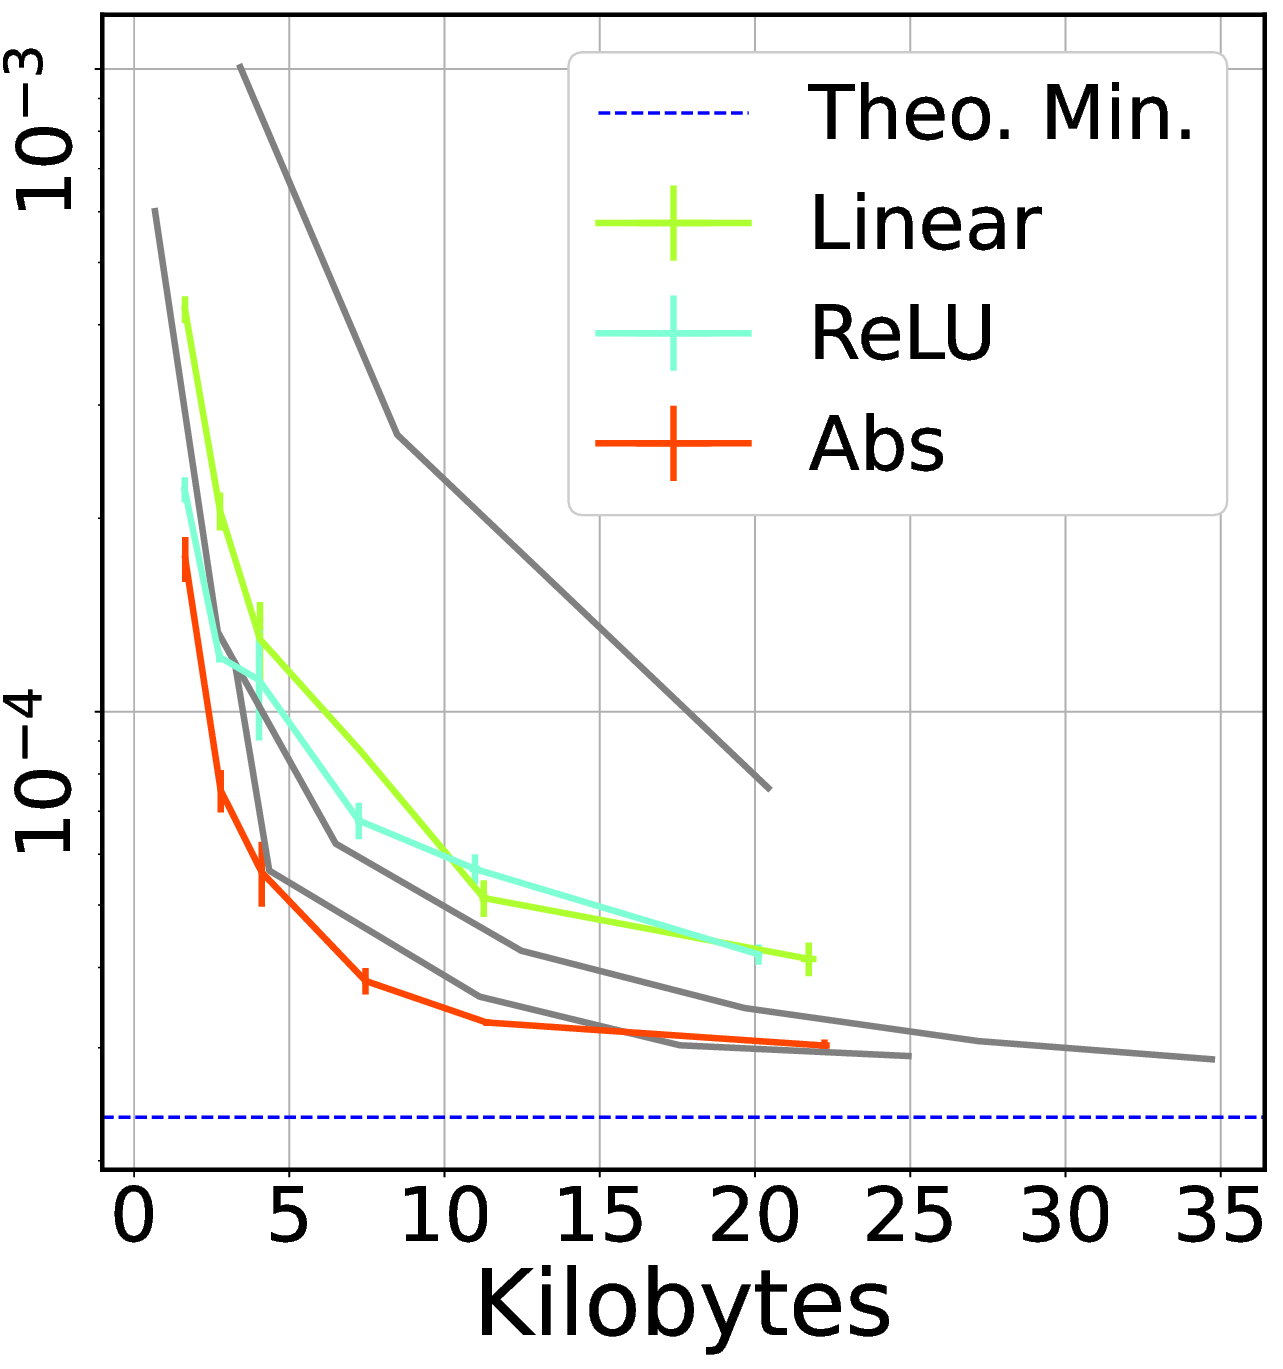} \\
a) Bitwidth $b$ &  b) $\lambda_{\ell 1}$  & c) UDF Activation \\
\end{tabular}
\caption{We analyze the impact of the quantization bitwidth $b$ (a), $\ell 1$-regularization (b) and the UDF activation function (c) on geometry compression on the Stanford shape repository~\cite{turk1994zippered}). In (a), we report the average \ac{cd} depending on the number of kilobytes for \acp{udf} using a bitwidth $\in \{ 6, 8, 10, 12 \}$. In (b), we report the average \ac{cd} depending on the number of kilobytes for \acp{udf} with ($\lambda_{\ell 1}=10^{-8}$) and without ($\lambda_{\ell 1}=0$) $\ell 1$-penalty. In (c), we report the average \ac{cd} depending on the number of kilobytes for \acp{udf} with linear, ReLU and abs activation function. We observe that using an abs activation drastically improves performance. We further depict Draco, GPCC and VPCC for reference in grey.}\label{fig:suppl_stanford_ablation}
\end{figure}

\begin{figure}[b!]
\centering
\setlength{\tabcolsep}{1pt}
\begin{tabular}{c}
\includegraphics[width=0.5\textwidth]{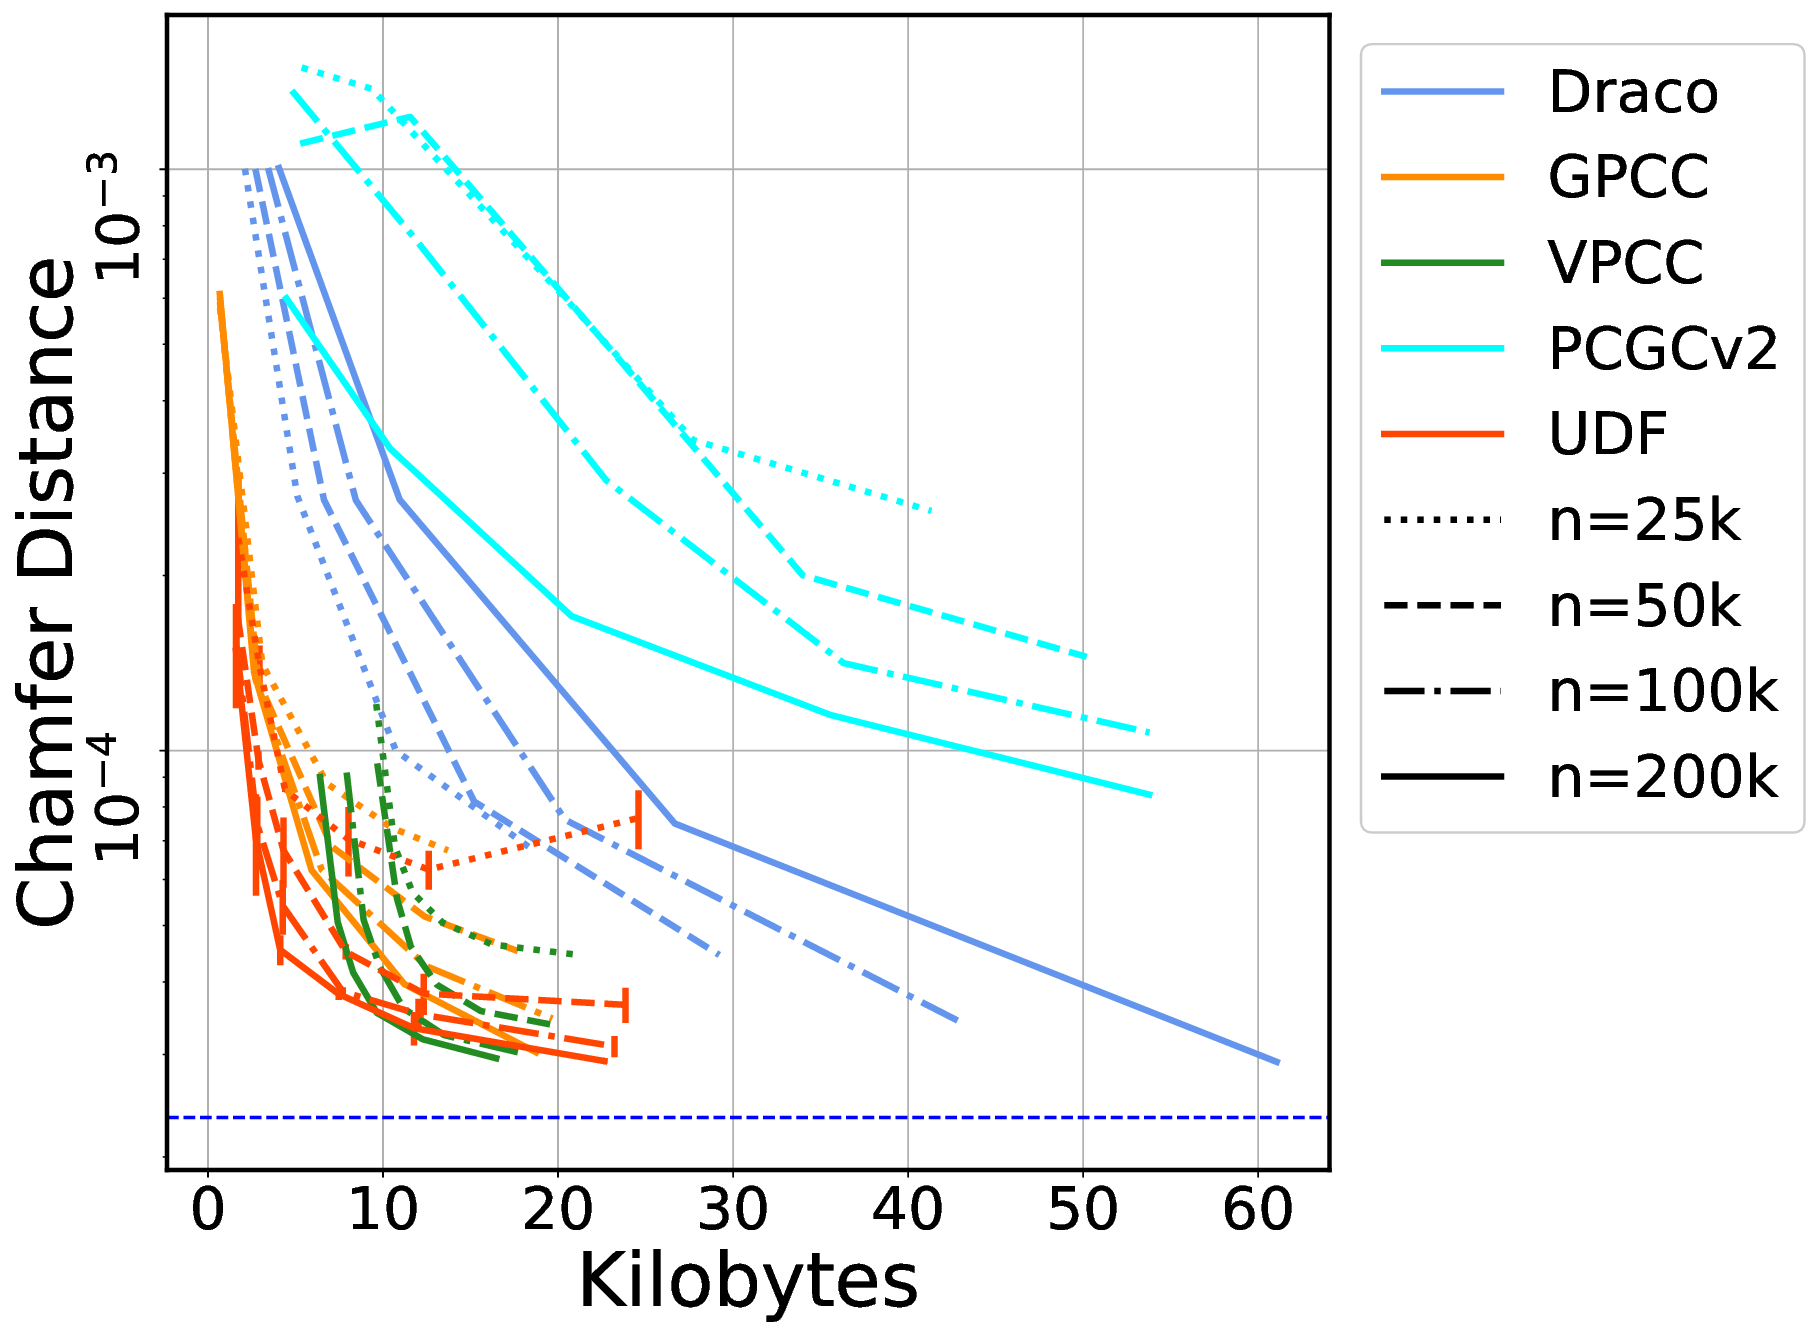} \\
\end{tabular}
\caption{We analyze the impact of the number of points in a \ac{pc} on geometry compression on the Stanford shape repository~\cite{turk1994zippered}). We conduct this analysis using Draco, \ac{gpcc}, \ac{vpcc}, \ac{pcgcv2} and \acp{udf} on the \stanford{}~\cite{turk1994zippered}. We use each method to compress \acp{pc} containing $n\in \{25k, 50k, 100k, 200k\}$ points. We perform evaluation using 100,000 points sampled from the ground truth to render the results comparable. We report the average \ac{cd} depending on the number of kilobytes. We observe that all methods, except for Draco, improve when the number of points increases.}\label{fig:suppl_number_of_points}
\end{figure}

\subsection{Bitwidth for Geometry Compression}\label{ssec:ablation_bitwidth}

We perform geometry compression using \acp{udf} on \attr{} with varying bitwidth $b\in\{6, 8, 10, 12\}$. \autoref{fig:suppl_stanford_ablation} (a) depicts the result. We find that $b=8$ yields the best performance. Smaller $b$ impact reconstruction performance too strongly. Larger $b$ do not further improve reconstruction performance, but increase the memory footprint of the model.

\subsection{$\ell 1$-Penalty on the Stanford Shape Repository}\label{ssec:ablation_l1}

In the main paper we demonstrated the impact of $\ell 1$-regularization on \attr{}. Here, we further show its impact on the \stanford{} by comparing the result of geometry compression using \acp{udf} with and without $\ell 1$-regularization. \autoref{fig:suppl_stanford_ablation} (b) shows the result. Using $\ell 1$-regularization reduces the impact of overfitting and, thus, improves the \ac{cd} at test time, resulting in a downwards shift of the RD curve. Furthermore, it renders the parameters of \acp{nf} more compressible, resulting in a leftwards shift. This effect can be best observed for larger models. 

\subsection{UDF Activation Function}\label{ssec:ablation_activation}

We proposed applying the abs activation function to the final output of \acp{udf} to render them more parameter efficient. In the main paper, we demonstrated that this drastically improves \acp{udf} on geometry compression when compared with a linear activation function. Chibane \etal~\cite{chibane2020neural}, who introduced \acp{udf}, proposed using a ReLU activation function instead. Therefore, we compare the ReLU, abs and linear activation function at this point. \autoref{fig:suppl_stanford_ablation} (c) depicts the result. We observe that the abs activation function improves performance on geometry compression significantly. For larger models the performance becomes more similar. In fact, the ReLU activation function performs similar to the linear activation function. This is reasonable since both functions are identical in the range of possible targets values of \acp{udf}.  

\subsection{Number of Points per Shape}\label{ssec:ablation_num_points}

We investigate the impact of the number of points in a \ac{pc} on the geometry compression performance of \ac{nf}-based compression using \acp{udf} and the baselines. To this end, we conduct experiments on the \stanford{}. We sample \acp{pc} from each shape with $n\in\{25K, 50K, 100K, 200K\}$ points. Then, we compress these and compare the reconstruction with $100K$ points sampled from the same shape. Using the same number of points for evaluation ensures comparability of the results. \autoref{fig:suppl_number_of_points} contains the result. We observe that all methods improve in terms of \ac{cd} when using more points which is expected. However, the memory foot print of Draco scales unfavourably when the number of points increases, whereas it remains approximately constant for other methods. \ac{gpcc} as well as \acp{udf} become more competitive with \ac{vpcc} when the number of points increases. \ac{pcgcv2} closes the gap to Draco.

\subsection{Joint Geometry and Attribute Compression}\label{ssec:ablation_geom_attr}

In this work, we first compress the geometry of 3D data and, then, compress its attributes given the learned geometry representation. Alternatively, one may also choose to learn a representation of the geometry and attributes simultaneously. This can be achieved by combining $\mathcal{L}_{G}$ and $\mathcal{L}_{A}$:
\begin{equation*}
    \mathcal{L}_{joint}(\theta) = \mathcal{L}_{G}(\theta) + \lambda_A \mathcal{L}_{A}(\theta)
\end{equation*}
Here, $\lambda_A$ quantifies the importance of the attribute reconstruction loss relative to the geometry reconstruction loss. We found empirically that $\lambda_A = 10^{-3}$ yields a good trade-off between geometry and attribute reconstruction. Further, note that in this case we fit a single \ac{nf} to represent the 3D data which could be potentially more parameter efficient. In contrast, in our approach one \ac{nf} represents the geometry and another one the attributes. Other training hyperparameters remain unchanged. \autoref{fig:suppl_attributes_ablation} (b) \& (c) depict the result.  We observe that using our approach (\ac{udf}/\ac{sdf} SEQ) both \acp{udf} and \acp{sdf} perform better that joint training (\ac{udf}/\ac{sdf} JOINT) on geometry as well as attribute compression. Merely, for strong compression ratios joint training yields a slightly smaller amount of kilobytes.  

\begin{figure}[t!]
\centering
\setlength{\tabcolsep}{1pt}
\begin{tabular}{ccc}
\includegraphics[width=\fourPlotsSizeWithLabel]{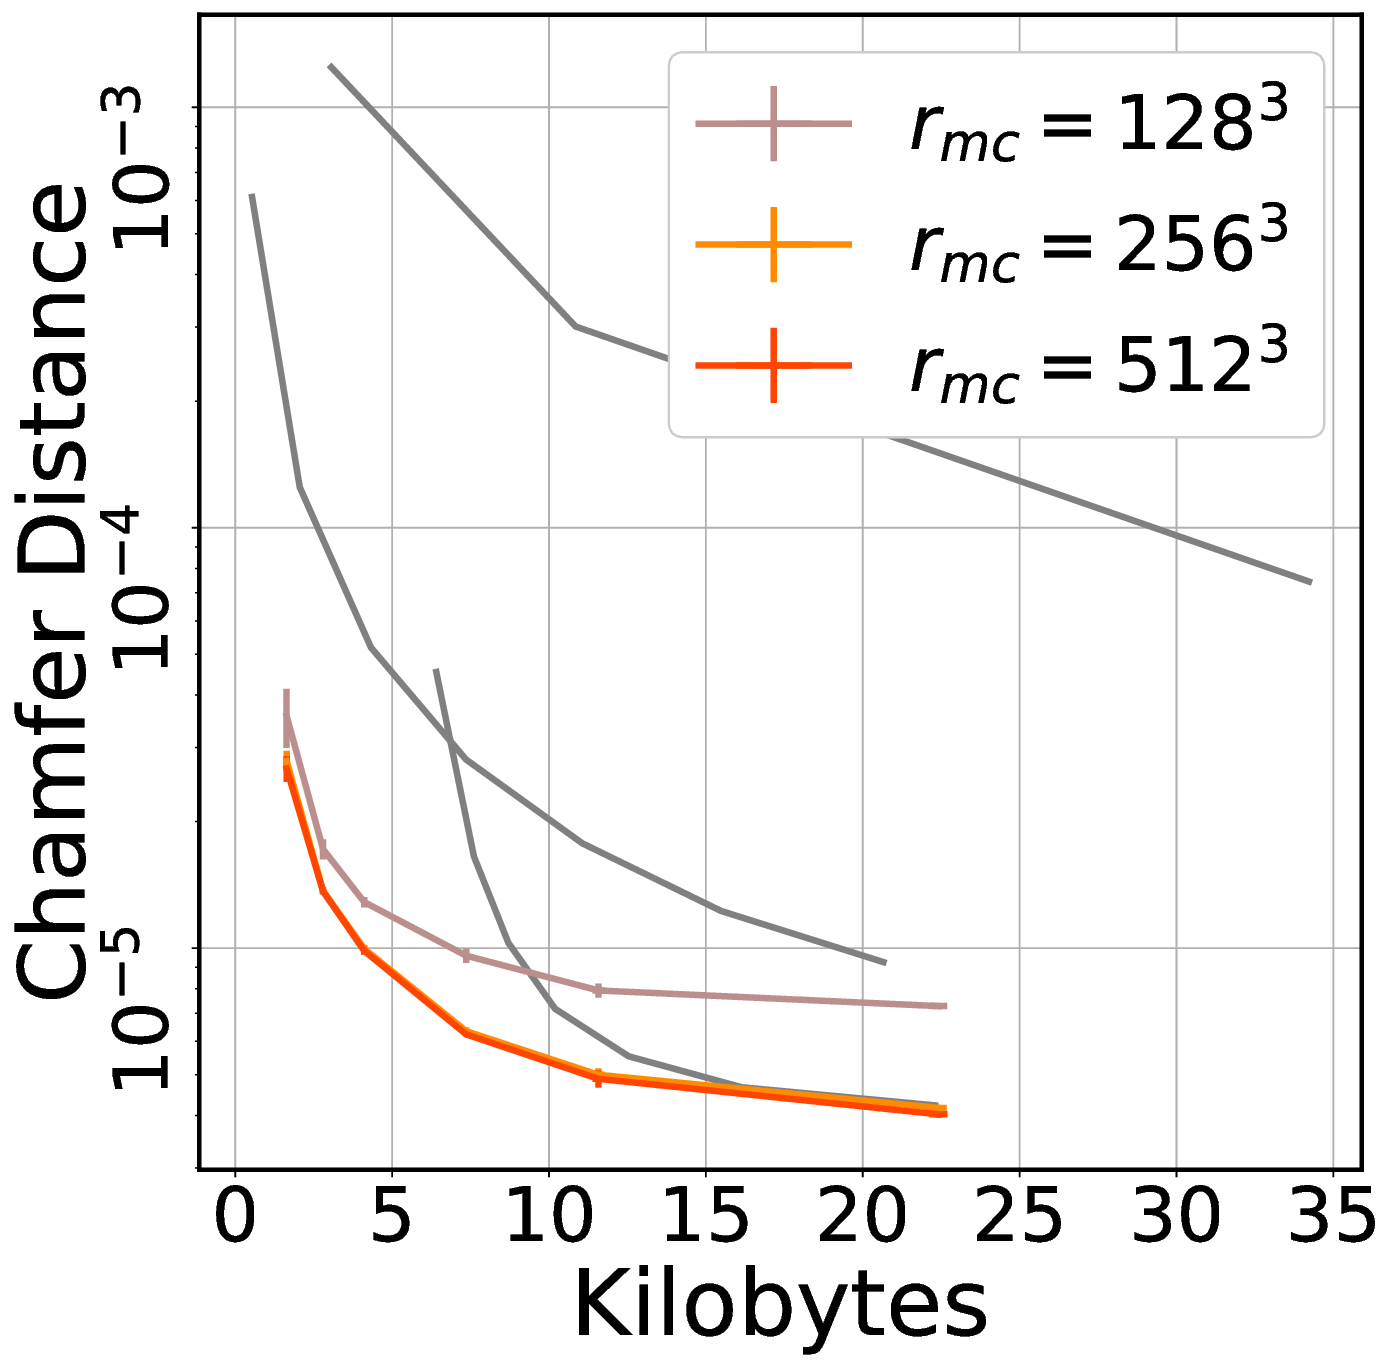} & 
\includegraphics[width=\fourPlotsSize]{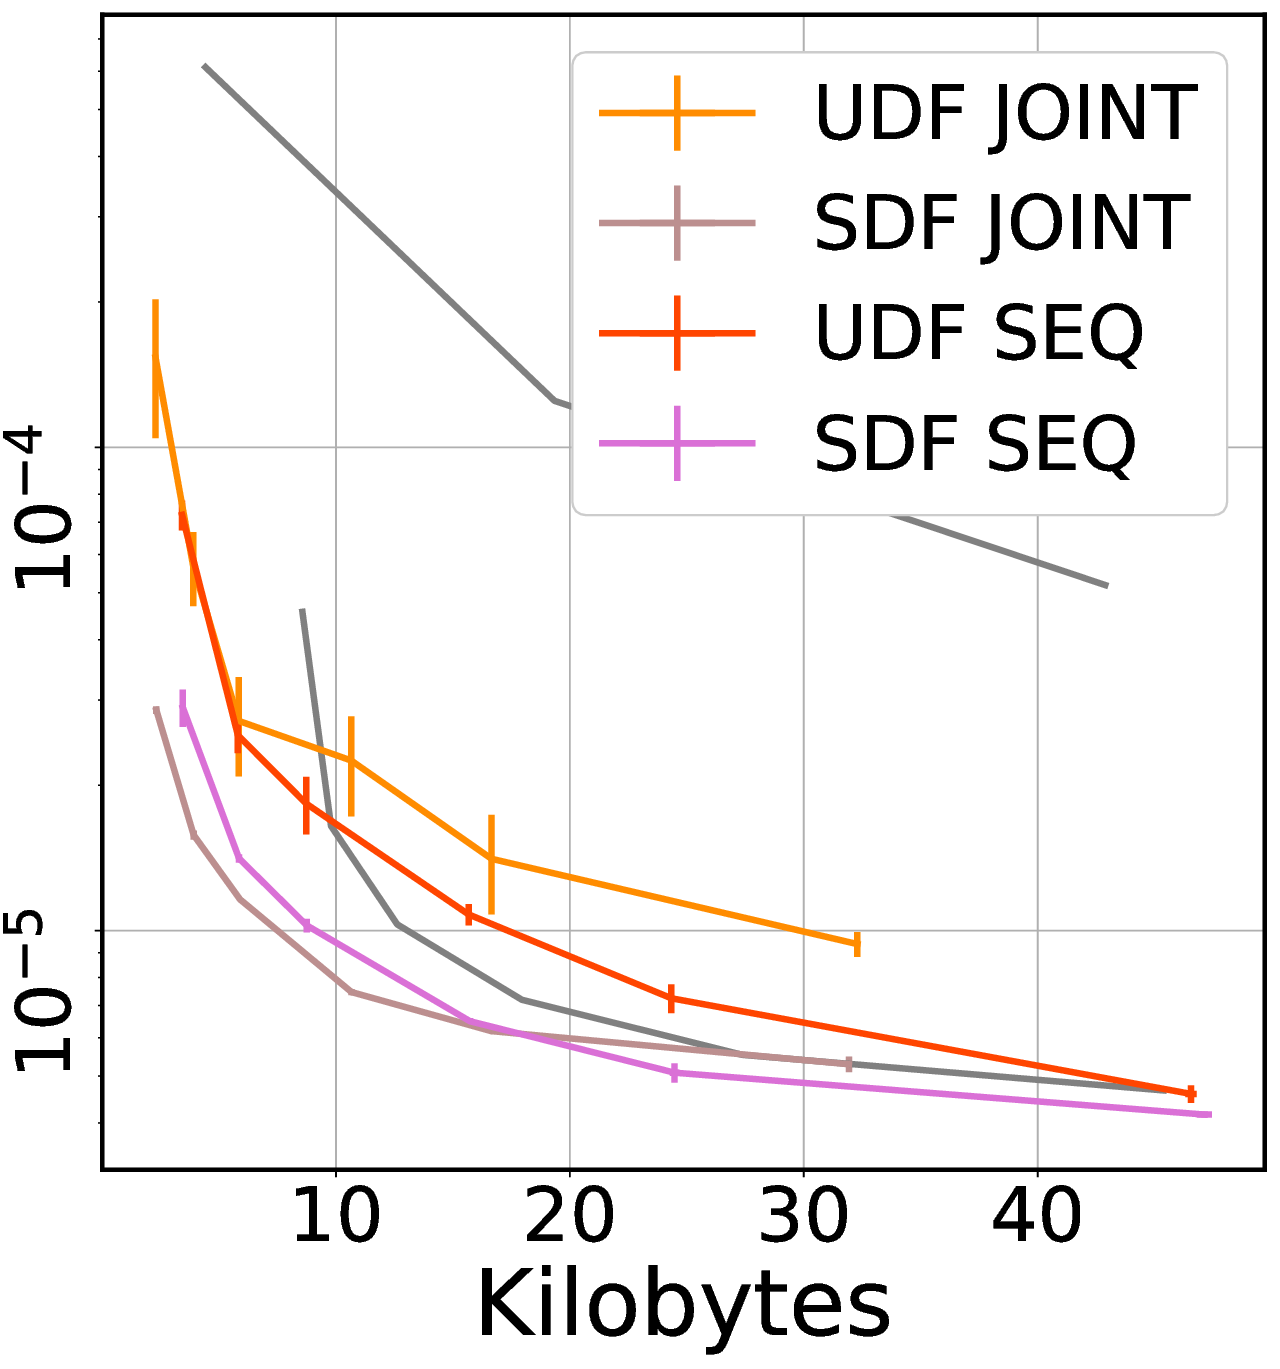} &
\includegraphics[width=\fourPlotsSizeWithLabel]{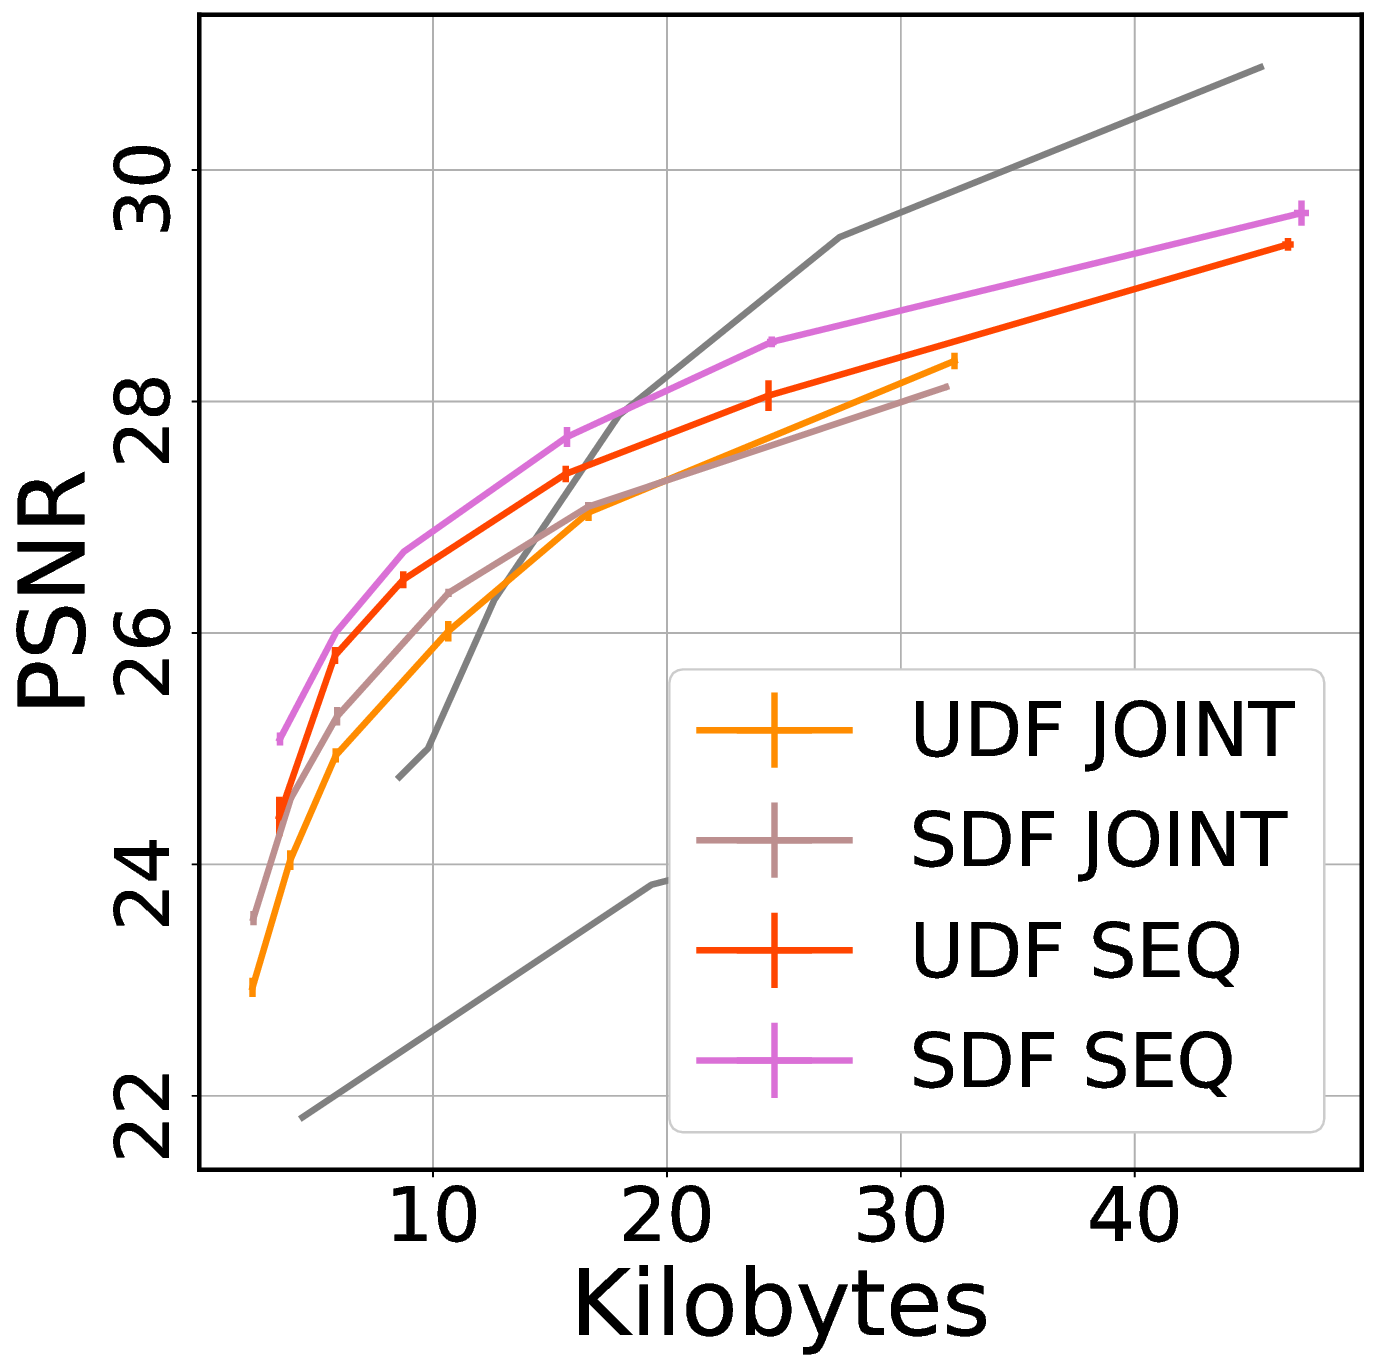} \\
a) \ac{mc} Grid Resolution &  b) Joint vs Seq. CD & c) Joint vs Seq. PSNR \\
\end{tabular}
\caption{We analyse the impact of the grid resolution used for \ac{mc} using \acp{sdf} (a) and compare jointly compressing geometry attributes with our proposed sequential approach on \attr{} (b/c). In (a), we observe that the largest performance gains are obtained when using a resolution of up to $256^3$. Afterwards, performance increase is diminishing. In (b/c), we report \ac{cd} on geometry compression (b) and \ac{psnr} for reconstructed color attributes (c). First compressing the geometry and, then, compressing color attributes (SDF/UDF SEQ) outperforms jointly learning to represent geometry and attributes (SDF/UDF JOINT).}\label{fig:suppl_attributes_ablation}
\end{figure}

\subsection{Grid Resolution used for Marching Cubes}\label{ssec:ablation_mc_grid}

When extracting meshes from \acp{nf}, we apply \ac{mc}~\cite{lorensen1987marching} (\acp{sdf}) or MeshUDF~\cite{guillard2022meshudf} (\acp{udf}). Both approaches require evaluating the \acp{nf} on a regular 3D grid in the area of interest. The resolution of this grid trades off reconstruction quality with runtime. Here, we evaluate the impact of changing the grid resolution $r_{mc}$ on the compression performance on \attr{} by evaluating \acp{sdf} for geometry compression using $r_{mc} \in \{128, 256, 512\}$. The result is depicted in \autoref{fig:suppl_attributes_ablation} (a). On \attr{}, we find that a resolution of $r_{mc} = 256$ is necessary to achieve competitive \ac{cd} performance. Note that $r_{mc}$ does not impact the file size of the compressed representation. Subsequently, performance gains from increasing $r_{mc}$ saturate.

\subsection{Fluctuation of Results Obtained Using UDFs}\label{ssec:udf_fluctuation}

We observe that the performance - particularly in terms of \ac{cd} - of \ac{nf}-based geometry compression using \acp{udf} fluctuates more strongly across independently trained models. Here, we investigate the root cause of this fluctuation. We identify two primary sources of randomness - the initialization of the dataset (\eg{} additive Gaussian noise) and the parameter initialization. In order to pinpoint the primary source, we train four different configurations with each 5 models on the \stanford{}: a) standard training without fixed random seeds, b) fixed random seed of dataset initialization, c) fixed random seed of parameter initialization and d) a) fixed random seeds of dataset and parameter initialization. \autoref{tab:suppl_fluctuation} contains the result of this analysis. We find that fixing the random seed of the parameter initialization has the strongest impact on the observed fluctuation. Note that we here measure the fluctuation as the mean standard deviation of the \ac{cd}. The mean is taken across different model sizes. 

\begin{table}[t!]
  \caption{We report the average standard deviation of the \ac{cd} across five independent trainings across all shapes in the Stanford shape repository. We either fix the parameter and/or the dataset initialization to investigate the root cause of the fluctuation of the compression performance of \acp{udf}. The fluctuation is measured as the average standard deviation across all compression ratios (\ie{} different model sizes). We observe that the parameter initialization has the largest impact on the fluctuation.}
  \label{tab:suppl_fluctuation}
  \centering
  \begin{tabular}{ccc}
    \toprule
    \multirow{2}{*}{\shortstack{Fixed parameter\\ initialization}}     & Fixed dataset     & $\sqrt{\textrm{Var}\left[\textrm{CD} \right]}$  \\
    &&\\
    \midrule
    \xmark & \xmark  & $7.5\times 10^-6$     \\
    \xmark & \cmark  & $5.6\times 10^-6$     \\
    \cmark & \xmark  & $2.5\times 10^-6$     \\
    \cmark & \cmark  & $1.5\times 10^-6$     \\
    \bottomrule
  \end{tabular}
\end{table}

\section{Experimental Details}\label{sec:experimental_details}

We provide additional experimental details of the training and evaluation of \acp{nf} (see \autoref{ssec:details_nf}) and the evaluation of the baselines (see \autoref{ssec:details_baselines}). We further describe how we extract meshes from \attr{} (see \autoref{ssec:details_meshes_attr}). 

\subsection{Neural Fields}\label{ssec:details_nf}

\paragraph{Positional Encodings.} We use almost the same positional enccodings as implemented in SIREN~\cite{sitzmann2020implicit}\footnote[1]{\url{https://github.com/vsitzmann/siren}}. Thus, we apply 
\begin{equation*}
\begin{split}
    \gamma (p) = & (p, \sin(\sigma_p^0 \pi p), \cos(\sigma_p^0 \pi p), \dots, \sin(\sigma_p^{L-1} \pi p), \cos(\sigma_p^{L-1} \pi p)).
\end{split}
\end{equation*}
separately to each dimension and concatenate the result. Compared to SIREN, we only add an additional scale parameter $\sigma_p$. We found that setting the scale parameter $\sigma_p=1.4$ works well across datasets. Further, we use $L=16$ for representing geometries and $L=8$ for color attributes.

\paragraph{Marching Cubes.} In order to extract meshes using \ac{mc}~\cite{lorensen1987marching} or MeshUDF~\cite{guillard2022meshudf}, we need to evaluate \acp{nf} on 3D regular grid in the region of interest. The resolution of the grid $r_{mc}$ trades off reconstruction quality with runtime. On \attr{}, we use $r_{mc}=512$ due to the large number of points in the \acp{pc} (see also \autoref{ssec:ablation_mc_grid}). We use $r_{mc}=256$ on the \stanford{} and the \garments{}. 

\subsection{Baselines}\label{ssec:details_baselines}

\paragraph{Draco}

We use the open source implementation of Draco~\footnote{\url{https://github.com/google/draco}}. Draco requires setting the parameters \textit{qp} and \textit{cl}. We set $cl=10$ which maximizes compression performance at the cost of decoding speed. We set $qp\in \{5, 6, 7\}$ to traverse the rate-distortion curve. 

\paragraph{GPCC}

\ac{gpcc} requires voxelized \acp{pc}. We achieve this for a given resolution $r_s$  by scaling the \acp{pc} with $r_s - 1$ and rounding to the nearest integer. 
\begin{equation*}
    x' =  \lfloor{(r_s-1)x}\rceil, \, y' = \lfloor{(r_s-1)y}\rceil, \, z'= \lfloor{(r_s-1)z}\rceil.
\end{equation*}
For \ac{gpcc}, we found that $r_s=1024$ worked best in the compression range in our experiments across datasets. For geometry compression we traverse the rate-distortion-curve using the position quantization scale $qs\in \{0.025, 0.055, 0.085, 0.115, 0.145, 0.175\}$. For attribute compression, we further trade off reconstruction quality with compression using the \textit{qp} parameter, $pq\in\{56, 51, 46\}$. When operating on \acp{pc} containing attributes, we also only use the first three values of \textit{qs} to land in the file size range of interest. We report further parameters used for attribute compression using \ac{gpcc} in \autoref{tab:suppl_further_gpcc_params}. All other parameters are set according to the official configuration file of the shape \textit{soldier} in \attr{}.

\begin{table}[t!]
  \caption{Further parameters used for attribute compression using \ac{gpcc}.}
  \label{tab:suppl_further_gpcc_params}
  \centering
  \begin{tabular}{cc}
    \toprule
    Parameter Name     & Value  \\
    \midrule
     \textit{adaptivePredictionThreshold}  & $64$     \\
     \textit{qpChromaOffset}  & $0$     \\
     \textit{bitdepth}  & $8$     \\
     \textit{attrOffset}  & $0$     \\
     \textit{attrScale}  & $1$     \\
     \textit{attribute}  & color     \\
    \bottomrule
  \end{tabular}
\end{table}

\paragraph{VPCC}

\ac{vpcc} requires voxelized \acp{pc}. Firstly, we translate and scale \acp{pc} using a scale $s$ and a translation t. We determine scale $s \in \mathbb{R}^3$ and translation $t \in \mathbb{R}^3$ as $t_i = \min_{x \in \mathcal{P}} \left[x_i\right]$ and $s_i = \max_{x \in \mathcal{P}}  \left[x_i\right] - t_i$. Intuitively, $t$ is the coordinate-wise smallest value and $s$ is the coordinate-wise largest elongation of the shape. Voxelization requires choosing a resolution of the voxel grid. We use the resolution $r_s=512$ which we found empirically to work well across datasets and in the file size range of interest. 
\begin{equation*}\label{eq:total_loss_geometry}
    x' =  \Bigg\lfloor{\dfrac{(r_s-1)(x - t)}{s}}\Bigg\rceil, \, y' = \Bigg\lfloor{\dfrac{(r_s-1)(y - t)}{s}}\Bigg\rceil, \, z'= \Bigg\lfloor{\dfrac{(r_s-1)(z - t)}{s}}\Bigg\rceil.
\end{equation*}
Here, each operation is element-wise. We trade off reconstruction quality with compression by varying the parameters (\textit{geometryQP}, \textit{occupancyPrecision}, \textit{attributeQP}) $\in \{(40, 4, 52), (36, 4, 47), (32, 4, 42), (28, 4, 37), (24, 4, 32), (20, 4, 27)\}$. These values are aligned with the official rates $\left[1-4\right]$ with a few points added in between to obtain more data points. The parameter \textit{attributeQP} is only used on \acp{pc} containing attributes to trade off reconstruction quality with compression for attributes.

\paragraph{PCGCv2}

PCGCv2 requires voxelized \acp{pc} as input. Thus, we adopt the preprocessing released in the official code repository of \ac{pcgcv2}\footnote{\url{https://github.com/NJUVISION/PCGCv2}}. We start with a normalized \ac{pc} $\mathcal{P}$, which can be either be obtained by sampling from the ground truth normalized mesh or by normalizing the ground truth \ac{pc}. We determine scale $s \in \mathbb{R}$ and translation $t \in \mathbb{R}$ as $t = \min_{(x,y,z) \in \mathcal{P}} \left[\min(\{x,y,z\})\right]$ and $s = \max_{(x,y,z) \in \mathcal{P}}  \left[\max(\{x,y,z\})\right] - t$. Intuitively, $t$ is the smallest coordinate for any point and axis and $s$ is the largest elongation of the shape in any axis. Voxelization requires choosing a resolution of the voxel grid. We use the resolution $r_s=1024$ as in the PCGCv2 paper. We then rescale according to
\begin{equation*}\label{eq:total_loss_geometry}
    x' =  \Bigg\lfloor{\dfrac{(r_s-1)(x - t)}{s}}\Bigg\rceil, \, y' = \Bigg\lfloor{\dfrac{(r_s-1)(y - t)}{s}}\Bigg\rceil, \, z'= \Bigg\lfloor{\dfrac{(r_s-1)(z - t)}{s}}\Bigg\rceil.
\end{equation*}
This results in the desired point cloud with coordinates as integer values in the range $[0, 1023]$. In our experiments, we found that it is very important to use this exact preprocessing. In fact, scaling each axis to [0, 1023] individually resulted in significantly worse compression results. Similarly, setting $t=0$ decreased performance noticeably. We evaluate PCGCv2 using the published model checkpoints for rates 1-5. Rate 1 corresponds to a target of 0.025 bpp (bits per point), whereas rate 5 corresponds to a target of 0.25 bpp.

\subsection{Meshes for 8iVFB}\label{ssec:details_meshes_attr}

\attr{} is comprised of \ac{pc}-attribute-pairs. However when training \acp{sdf}, we require meshes to determine the sign of the distance. Therefore, we extract meshes from the \acp{pc} in \attr{} using Poisson surface reconstruction~\cite{kazhdan2006poisson}. We use the open3d implementation~\cite{Zhou2018}. We set the depth of Poisson surface reconstruction to 9. Normals of the \acp{pc}, which are a prerequisite for surface reconstruction, are estimated using local PCA and oriented using 20 nearest neighbors.

\section{Qualitative Results}\label{sec:qualitative_results}

We show additional qualitative examples in this section. \autoref{ssec:qualitative_stanford} shows qualitative exmaples of reconstructed \acp{pc} on the \stanford{}. \autoref{ssec:qualitative_garments} depicts reconstructed meshes on the \garments{}. Lastly, \autoref{ssec:qualitative_attr} contains reconstructed \acp{pc} including their attributes on \attr{}. Reported kilobytes refer to the average across the dataset at a particular rate for each compression algorithm.

\subsection{Point Cloud Geometry Compression on the Stanford Shape Repository}\label{ssec:qualitative_stanford}

\autoref{fig:suppl_qualitative_stanford} depicts reconstructions of \acp{pc} for the remaining shapes of the \stanford{}. We visualize Draco, \ac{gpcc}, \ac{vpcc}, \ac{pcgcv2}, \acp{udf}, \acp{sdf} and the ground truth.

\begin{figure}
% NOTE: stanfordPCQualitativeFigWidthSuppl is defined in custom/commands.tex
\centering
    \begin{tabular}{ccccccc}   
    \small a) Draco & b) \ac{pcgcv2} & c) GPCC & d) VPCC & e) UDF & f) SDF & g) GT\\
    \small 9.2 KB & \small 11.8 KB & \small 4.8 KB & \small 8.0 KB & \small 4.2 KB & \small 4.2 KB & \small 2.9 MB \\
    \includegraphics[width=\stanfordPCQualitativeFigWidthSuppl]{figs/qualitative_examples/stanfordshapes_normalized_rec/draco_6_rendered/bun_zipper_crop.eps}
    & \includegraphics[width=\stanfordPCQualitativeFigWidthSuppl]{figs/qualitative_examples/stanfordshapes_normalized_rec/lpcgc_dset_stanfordshapes_normalized_pc_100000_eval_100000_scale_1024/1_corrected_rendered/bun_zipper_dec_crop.eps}
    & \includegraphics[width=\stanfordPCQualitativeFigWidthSuppl]{figs/qualitative_examples/stanfordshapes_normalized_rec/gpcc_0.085_46_rendered/bun_zipper_crop.eps} & 
    \includegraphics[width=\stanfordPCQualitativeFigWidthSuppl]{figs/qualitative_examples/stanfordshapes_normalized_rec/vpcc_40_4_rendered/bun_zipper_dec_crop.eps} &
    \includegraphics[width=\stanfordPCQualitativeFigWidthSuppl]{figs/qualitative_examples/stanfordshapes_normalized_rec/udf_32_rendered/bun_zipper_crop.eps} & \includegraphics[width=\stanfordPCQualitativeFigWidthSuppl]{figs/qualitative_examples/stanfordshapes_normalized_rec/sdf_32_rendered/bun_zipper_crop.eps} &\includegraphics[width=\stanfordPCQualitativeFigWidthSuppl]{figs/qualitative_examples/datasets/stanfordshapes_normalized/bun_zipper_num_points_100000_crop.eps}\\
    \end{tabular}
    \begin{tabular}{ccccccc}  
    \includegraphics[width=\stanfordPCQualitativeFigWidthSuppl]{figs/qualitative_examples/stanfordshapes_normalized_rec/draco_6_rendered/dragon_vrip_dec_crop.eps} & \includegraphics[width=\stanfordPCQualitativeFigWidthSuppl]{figs/qualitative_examples/stanfordshapes_normalized_rec/lpcgc_dset_stanfordshapes_normalized_pc_100000_eval_100000_scale_1024/1_corrected_rendered/dragon_vrip_dec_crop.eps} & \includegraphics[width=\stanfordPCQualitativeFigWidthSuppl]{figs/qualitative_examples/stanfordshapes_normalized_rec/gpcc_0.085_46_rendered/dragon_vrip_dec_crop.eps} & 
    \includegraphics[width=\stanfordPCQualitativeFigWidthSuppl]{figs/qualitative_examples/stanfordshapes_normalized_rec/vpcc_40_4_rendered/dragon_vrip_dec_crop.eps} &
    \includegraphics[width=\stanfordPCQualitativeFigWidthSuppl]{figs/qualitative_examples/stanfordshapes_normalized_rec/udf_32_rendered/dragon_vrip_crop.eps} & \includegraphics[width=\stanfordPCQualitativeFigWidthSuppl]{figs/qualitative_examples/stanfordshapes_normalized_rec/sdf_32_rendered/dragon_vrip_crop.eps} &\includegraphics[width=\stanfordPCQualitativeFigWidthSuppl]{figs/qualitative_examples/datasets/stanfordshapes_normalized/dragon_vrip_num_points_100000_crop.eps}\\
    \end{tabular}
    \begin{tabular}{ccccccc}  
    \includegraphics[width=\stanfordPCQualitativeFigWidthSuppl]{figs/qualitative_examples/stanfordshapes_normalized_rec/draco_6_rendered/happy_vrip_dec_crop.eps}
    & \includegraphics[width=\stanfordPCQualitativeFigWidthSuppl]{figs/qualitative_examples/stanfordshapes_normalized_rec/lpcgc_dset_stanfordshapes_normalized_pc_100000_eval_100000_scale_1024/1_corrected_rendered/happy_vrip_dec_crop.eps} & \includegraphics[width=\stanfordPCQualitativeFigWidthSuppl]{figs/qualitative_examples/stanfordshapes_normalized_rec/gpcc_0.085_46_rendered/happy_vrip_dec_crop.eps} & 
    \includegraphics[width=\stanfordPCQualitativeFigWidthSuppl]{figs/qualitative_examples/stanfordshapes_normalized_rec/vpcc_40_4_rendered/happy_vrip_dec_crop.eps} &
    \includegraphics[width=\stanfordPCQualitativeFigWidthSuppl]{figs/qualitative_examples/stanfordshapes_normalized_rec/udf_32_rendered/happy_vrip_crop.eps} & \includegraphics[width=\stanfordPCQualitativeFigWidthSuppl]{figs/qualitative_examples/stanfordshapes_normalized_rec/sdf_32_rendered/happy_vrip_crop.eps} &\includegraphics[width=\stanfordPCQualitativeFigWidthSuppl]{figs/qualitative_examples/datasets/stanfordshapes_normalized/happy_vrip_num_points_100000_crop.eps}\\
    \end{tabular}
    \begin{tabular}{ccccccc}  
    \includegraphics[scale=.2]{figs/qualitative_examples/stanfordshapes_normalized_rec/draco_6_rendered/drill_shaft_vrip_dec_crop.eps} 
    & \includegraphics[scale=.2]{figs/qualitative_examples/stanfordshapes_normalized_rec/lpcgc_dset_stanfordshapes_normalized_pc_100000_eval_100000_scale_1024/1_corrected_rendered/drill_shaft_vrip_dec_crop.eps} & \includegraphics[scale=.2]{figs/qualitative_examples/stanfordshapes_normalized_rec/gpcc_0.085_46_rendered/drill_shaft_vrip_dec_crop.eps} & 
    \includegraphics[scale=.2]{figs/qualitative_examples/stanfordshapes_normalized_rec/vpcc_40_4_rendered/drill_shaft_vrip_dec_crop.eps} &
    \includegraphics[scale=.2]{figs/qualitative_examples/stanfordshapes_normalized_rec/udf_32_rendered/drill_shaft_vrip_crop.eps} & \includegraphics[scale=.2]{figs/qualitative_examples/stanfordshapes_normalized_rec/sdf_32_rendered/drill_shaft_vrip_crop.eps} &\includegraphics[scale=.2]{figs/qualitative_examples/datasets/stanfordshapes_normalized/drill_shaft_vrip_num_points_100000_crop.eps}\\
    \end{tabular}
    % \begin{tabular}{ccccccc}  
    % \includegraphics[width=\stanfordPCQualitativeFigWidthSuppl]{figs/qualitative_examples/stanfordshapes_normalized_rec/draco_6_rendered/lucy_normalized_dec_crop.eps} 
    % & \includegraphics[width=\stanfordPCQualitativeFigWidthSuppl]{figs/qualitative_examples/stanfordshapes_normalized_rec/lpcgc_dset_stanfordshapes_normalized_pc_100000_eval_100000_scale_1024/1_corrected_rendered/lucy_normalized_dec_crop.eps} & \includegraphics[width=\stanfordPCQualitativeFigWidthSuppl]{figs/qualitative_examples/stanfordshapes_normalized_rec/gpcc_0.085_46_rendered/lucy_normalized_dec_crop.eps} & 
    % \includegraphics[width=\stanfordPCQualitativeFigWidthSuppl]{figs/qualitative_examples/stanfordshapes_normalized_rec/vpcc_40_4_rendered/lucy_normalized_dec_crop.eps} &
    % \includegraphics[width=\stanfordPCQualitativeFigWidthSuppl]{figs/qualitative_examples/stanfordshapes_normalized_rec/udf_32_rendered/lucy_normalized_crop.eps} & \includegraphics[width=\stanfordPCQualitativeFigWidthSuppl]{figs/qualitative_examples/stanfordshapes_normalized_rec/sdf_32_rendered/lucy_normalized_crop.eps} &\includegraphics[width=\stanfordPCQualitativeFigWidthSuppl]{figs/qualitative_examples/datasets/stanfordshapes_normalized/lucy_normalized_num_points_100000_crop.eps}\\ \small a) Draco & b) \ac{pcgcv2} & c) GPCC & d) VPCC & e) UDF & f) SDF & g) GT\\
    % \end{tabular}
    \caption{Qualitative examples of reconstructed \acp{pc} on the \stanford{}.}\label{fig:suppl_qualitative_stanford}
\end{figure}

\begin{figure}
% NOTE: stanfordPCQualitativeFigWidthSuppl is defined in custom/commands.tex
\centering
\begin{tabular}{ccccccc}  
    \small a) Draco & b) \ac{pcgcv2} & c) GPCC & d) VPCC & e) UDF & f) SDF & g) GT\\
    \small 9.2 KB & \small 11.8 KB & \small 4.8 KB & \small 8.0 KB & \small 4.2 KB & \small 4.2 KB & \small 2.9 MB \\
    \includegraphics[width=\stanfordPCQualitativeFigWidthSuppl]{figs/qualitative_examples/stanfordshapes_normalized_rec/draco_6_rendered/lucy_normalized_dec_crop.eps} 
    & \includegraphics[width=\stanfordPCQualitativeFigWidthSuppl]{figs/qualitative_examples/stanfordshapes_normalized_rec/lpcgc_dset_stanfordshapes_normalized_pc_100000_eval_100000_scale_1024/1_corrected_rendered/lucy_normalized_dec_crop.eps} & \includegraphics[width=\stanfordPCQualitativeFigWidthSuppl]{figs/qualitative_examples/stanfordshapes_normalized_rec/gpcc_0.085_46_rendered/lucy_normalized_dec_crop.eps} & 
    \includegraphics[width=\stanfordPCQualitativeFigWidthSuppl]{figs/qualitative_examples/stanfordshapes_normalized_rec/vpcc_40_4_rendered/lucy_normalized_dec_crop.eps} &
    \includegraphics[width=\stanfordPCQualitativeFigWidthSuppl]{figs/qualitative_examples/stanfordshapes_normalized_rec/udf_32_rendered/lucy_normalized_crop.eps} & \includegraphics[width=\stanfordPCQualitativeFigWidthSuppl]{figs/qualitative_examples/stanfordshapes_normalized_rec/sdf_32_rendered/lucy_normalized_crop.eps} &\includegraphics[width=\stanfordPCQualitativeFigWidthSuppl]{figs/qualitative_examples/datasets/stanfordshapes_normalized/lucy_normalized_num_points_100000_crop.eps}\\
    \end{tabular}
\begin{tabular}{ccccccc}  
    \includegraphics[width=\stanfordPCQualitativeFigWidthSuppl]{figs/qualitative_examples/stanfordshapes_normalized_rec/draco_6_rendered/xyzrgb_dragon_normalized_dec_crop.eps} & \includegraphics[width=\stanfordPCQualitativeFigWidthSuppl]{figs/qualitative_examples/stanfordshapes_normalized_rec/lpcgc_dset_stanfordshapes_normalized_pc_100000_eval_100000_scale_1024/1_corrected_rendered/xyzrgb_dragon_normalized_dec_crop.eps} & \includegraphics[width=\stanfordPCQualitativeFigWidthSuppl]{figs/qualitative_examples/stanfordshapes_normalized_rec/gpcc_0.085_46_rendered/xyzrgb_dragon_normalized_dec_crop.eps} & 
    \includegraphics[width=\stanfordPCQualitativeFigWidthSuppl]{figs/qualitative_examples/stanfordshapes_normalized_rec/vpcc_40_4_rendered/xyzrgb_dragon_normalized_dec_crop.eps} &
    \includegraphics[width=\stanfordPCQualitativeFigWidthSuppl]{figs/qualitative_examples/stanfordshapes_normalized_rec/udf_32_rendered/xyzrgb_dragon_normalized_crop.eps} & \includegraphics[width=\stanfordPCQualitativeFigWidthSuppl]{figs/qualitative_examples/stanfordshapes_normalized_rec/sdf_32_rendered/xyzrgb_dragon_normalized_crop.eps} &\includegraphics[width=\stanfordPCQualitativeFigWidthSuppl]{figs/qualitative_examples/datasets/stanfordshapes_normalized/xyzrgb_dragon_normalized_num_points_100000_crop.eps}\\ 
    \end{tabular}
    \begin{tabular}{ccccccc}  
    \includegraphics[width=\stanfordPCQualitativeFigWidthSuppl]{figs/qualitative_examples/stanfordshapes_normalized_rec/draco_6_rendered/xyzrgb_manuscript_dec_crop.eps} & 
    \includegraphics[width=\stanfordPCQualitativeFigWidthSuppl]{figs/qualitative_examples/stanfordshapes_normalized_rec/lpcgc_dset_stanfordshapes_normalized_pc_100000_eval_100000_scale_1024/1_corrected_rendered/xyzrgb_manuscript_dec_crop.eps} & \includegraphics[width=\stanfordPCQualitativeFigWidthSuppl]{figs/qualitative_examples/stanfordshapes_normalized_rec/gpcc_0.085_46_rendered/xyzrgb_manuscript_dec_crop.eps} & 
    \includegraphics[width=\stanfordPCQualitativeFigWidthSuppl]{figs/qualitative_examples/stanfordshapes_normalized_rec/vpcc_40_4_rendered/xyzrgb_manuscript_dec_crop.eps} &
    \includegraphics[width=\stanfordPCQualitativeFigWidthSuppl]{figs/qualitative_examples/stanfordshapes_normalized_rec/udf_32_rendered/xyzrgb_manuscript_crop.eps} & \includegraphics[width=\stanfordPCQualitativeFigWidthSuppl]{figs/qualitative_examples/stanfordshapes_normalized_rec/sdf_32_rendered/xyzrgb_manuscript_crop.eps} &\includegraphics[width=\stanfordPCQualitativeFigWidthSuppl]{figs/qualitative_examples/datasets/stanfordshapes_normalized/xyzrgb_manuscript_num_points_100000_crop.eps}\\
    \end{tabular}
    \begin{tabular}{ccccccc}  
    \includegraphics[width=\stanfordPCQualitativeFigWidthSuppl]{figs/qualitative_examples/stanfordshapes_normalized_rec/draco_6_rendered/xyzrgb_statuette_normalized_dec_crop.eps} & 
    \includegraphics[width=\stanfordPCQualitativeFigWidthSuppl]{figs/qualitative_examples/stanfordshapes_normalized_rec/lpcgc_dset_stanfordshapes_normalized_pc_100000_eval_100000_scale_1024/1_corrected_rendered/xyzrgb_statuette_normalized_dec_crop.eps} &
    \includegraphics[width=\stanfordPCQualitativeFigWidthSuppl]{figs/qualitative_examples/stanfordshapes_normalized_rec/gpcc_0.085_46_rendered/xyzrgb_statuette_normalized_dec_crop.eps} & 
    \includegraphics[width=\stanfordPCQualitativeFigWidthSuppl]{figs/qualitative_examples/stanfordshapes_normalized_rec/vpcc_40_4_rendered/xyzrgb_statuette_normalized_dec_crop.eps} &
    \includegraphics[width=\stanfordPCQualitativeFigWidthSuppl]{figs/qualitative_examples/stanfordshapes_normalized_rec/udf_32_rendered/xyzrgb_statuette_normalized_crop.eps} & \includegraphics[width=\stanfordPCQualitativeFigWidthSuppl]{figs/qualitative_examples/stanfordshapes_normalized_rec/sdf_32_rendered/xyzrgb_statuette_normalized_crop.eps} &\includegraphics[width=\stanfordPCQualitativeFigWidthSuppl]{figs/qualitative_examples/datasets/stanfordshapes_normalized/xyzrgb_statuette_normalized_num_points_100000_crop.eps}\\ 
    \end{tabular}
    \caption{Qualitative examples of reconstructed \acp{pc} on the \stanford{} part two .}\label{fig:suppl_qualitative_stanford_2}
\end{figure}

\subsection{Mesh Compression on the MGN Dataset}\label{ssec:qualitative_garments}

\autoref{fig:suppl_qualitative_garments} shows qualitative examples of reconstructed meshes on the \garments{}. We visualize reconstructions for Draco, \acp{udf} and the ground truth.

\begin{figure}
\centering
    \begin{tabular}{ccc}   
    \small a) Draco (4.8 KB) & b) \ac{udf} (7.5 KB) & c) GT (307 KB)\\
    \includegraphics[width=\meshQualitativeFigWidthGarments]{figs/qualitative_examples/garments_normalized_subset_rec_rendered/draco_7_mesh_rendered/Pants_125611494277906_crop.eps} & \includegraphics[width=\meshQualitativeFigWidthGarments]{figs/qualitative_examples/garments_normalized_subset_rec_rendered/udf_48_mesh_rendered/Pants_125611494277906_mesh_crop.eps} & \includegraphics[width=\meshQualitativeFigWidthGarments]{figs/qualitative_examples/datasets/garments_normalized_subset_rendered/Pants_125611494277906_crop.eps}\\ 
    \end{tabular}%
    \newline
    \begin{tabular}{ccc}                              \includegraphics[width=\meshQualitativeFigWidthGarments]{figs/qualitative_examples/garments_normalized_subset_rec_rendered/draco_7_mesh_rendered/ShirtNoCoat_125611521914479_dec_crop.eps} & \includegraphics[width=\meshQualitativeFigWidthGarments]{figs/qualitative_examples/garments_normalized_subset_rec_rendered/udf_48_mesh_rendered/ShirtNoCoat_125611521914479_mesh_crop.eps} & \includegraphics[width=\meshQualitativeFigWidthGarments]{figs/qualitative_examples/datasets/garments_normalized_subset_rendered/ShirtNoCoat_125611521914479_crop.eps}\\
    \end{tabular}%
    \newline
    \begin{tabular}{ccc}
    \hspace{-18mm}
    \includegraphics[width=\meshQualitativeFigWidthGarments]{figs/qualitative_examples/garments_normalized_subset_rec_rendered/draco_7_mesh_rendered/ShortPants_125611499279708_dec_crop.eps} & \includegraphics[width=\meshQualitativeFigWidthGarments]{figs/qualitative_examples/garments_normalized_subset_rec_rendered/udf_48_mesh_rendered/ShortPants_125611499279708_mesh_crop.eps} & \includegraphics[width=\meshQualitativeFigWidthGarments]{figs/qualitative_examples/datasets/garments_normalized_subset_rendered/ShortPants_125611499279708_crop.eps}\\ 
    \end{tabular}%
    \caption{Qualitative examples of reconstructed meshes on the \garments{}.}\label{fig:suppl_qualitative_garments}
\end{figure}

\subsection{Point Cloud Geomtry \& Attribute Compression on 8i Voxelized Full Bodies}\label{ssec:qualitative_attr}

\autoref{fig:suppl_qualitative_attr} depicts qualitative examples of the additional shapes of \attr{}.

\begin{figure}
\centering
    \begin{tabular}{ccccc}   
    \small a) GPCC (19.3 KB) & \small b) VPCC (18.0 KB) & \small c) \ac{udf} (15.7 KB) & \small d) \ac{sdf} (15.7 KB) & \small e) GT (20.2 MB)\\
    \includegraphics[width=\attributesPCQualitativeFigWidthSuppl]{figs/qualitative_examples/attribute_pcs_normalized_rec/gpcc_0.055_51/loot_dec_crop.eps} & \includegraphics[width=\attributesPCQualitativeFigWidthSuppl]{figs/qualitative_examples/attribute_pcs_normalized_rec/vpcc_36_4_attr/loot_dec_crop.eps} & \includegraphics[width=\attributesPCQualitativeFigWidthSuppl]{figs/qualitative_examples/attribute_pcs_normalized_rec/udf_64_attr/loot_crop.eps} & \includegraphics[width=\attributesPCQualitativeFigWidthSuppl]{figs/qualitative_examples/attribute_pcs_normalized_rec/sdf_64_attr/loot_crop.eps} & \includegraphics[width=\attributesPCQualitativeFigWidthSuppl]{figs/qualitative_examples/datasets/attributes_pcs_normalized_rendered/loot_crop.eps}
    \\ 
    % \end{tabular}
    % \end{figure}
    % \begin{figure}[H]
    % \centering
    % \begin{tabular}{ccccc} 
    \includegraphics[width=\attributesPCQualitativeFigWidthSuppl]{figs/qualitative_examples/attribute_pcs_normalized_rec/gpcc_0.055_51/redandblack_dec_crop.eps} & \includegraphics[width=\attributesPCQualitativeFigWidthSuppl]{figs/qualitative_examples/attribute_pcs_normalized_rec/vpcc_36_4_attr/redandblack_dec_crop.eps} & \includegraphics[width=\attributesPCQualitativeFigWidthSuppl]{figs/qualitative_examples/attribute_pcs_normalized_rec/udf_64_attr/redandblack_crop.eps} & \includegraphics[width=\attributesPCQualitativeFigWidthSuppl]{figs/qualitative_examples/attribute_pcs_normalized_rec/sdf_64_attr/redandblack_crop.eps} & \includegraphics[width=\attributesPCQualitativeFigWidthSuppl]{figs/qualitative_examples/datasets/attributes_pcs_normalized_rendered/redandblack_crop.eps}\\
    % \end{tabular}
    % \end{figure}
    % \begin{figure}[H]
    % \centering
    % \begin{tabular}{ccccc} 
    \includegraphics[width=\attributesPCQualitativeFigWidthSuppl]{figs/qualitative_examples/attribute_pcs_normalized_rec/gpcc_0.055_51/soldier_dec_crop.eps} & \includegraphics[width=\attributesPCQualitativeFigWidthSuppl]{figs/qualitative_examples/attribute_pcs_normalized_rec/vpcc_36_4_attr/soldier_dec_crop.eps} & \includegraphics[width=\attributesPCQualitativeFigWidthSuppl]{figs/qualitative_examples/attribute_pcs_normalized_rec/udf_64_attr/soldier_crop.eps} & \includegraphics[width=\attributesPCQualitativeFigWidthSuppl]{figs/qualitative_examples/attribute_pcs_normalized_rec/sdf_64_attr/soldier_crop.eps} & \includegraphics[width=\attributesPCQualitativeFigWidthSuppl]{figs/qualitative_examples/datasets/attributes_pcs_normalized_rendered/soldier_crop.eps}\\ 
    \end{tabular}
    \caption{Qualitative examples of reconstructed \acp{pc} including their attributes on \attr{}.}\label{fig:suppl_qualitative_attr}
\end{figure}
